# Supplementary material for: Chorus: a Programming Framework for Building Scalable Differential Privacy Mechanisms
Source: arXiv:1809.07750 source file (2021-05-04)
Supplement: Supplementary file 1 [file appendix-figures.tex]

\section{Additional Query Rewriting Definitions}
\label{sec:addit-query-rewr}

\begin{figure*}
  \centering
\begin{lstlisting}[frame=single]
(*@ \fbox{\emph{IQR}} @*)(<N>, <T>, (*@ $n$ @*))
\end{lstlisting}
$\Downarrow$
\begin{lstlisting}[frame=single]
WITH
  -- get private quantiles
  -- get common metrics for the list
  pq1 as (select <N> from <T> order by <N>),
  pq2 as (select *, row_number() as idx from pq1),
  pq_common as (select a.<N> as Zi, b.<N> as Zi1, b.idx as i from pq2 a inner join pq2 b on a.idx+1 = b.idx),
  
  -- get the min
  pq4_min as (select Zi1, Zi, (Zi1 - Zi) * EXP(-1*ABS(i-0.1*9)) as Yi, i from pq_common),
  pq4sum_min as (select sum(Yi) as sumYi from pq4_min),
  pq5_min as (select *, Yi/sumYi as probYi, random() as rand from pq4_min cross join pq4sum_min),
  pq6_min as (select Zi1, Zi, i, rand < probYi as picked from pq5_min),
  pq6zero_min as (select min(Zi) as Zi1, 0 as Zi, 1 as i, true as picked from pq6_min),
  pq6with1_min as (select * from pq6_min union select * from pq6zero_min order by i asc),
  pq7_min as (select random()*(Zi1-Zi)+Zi as priv_min from pq6with1_min where picked is true order by i desc limit 1),
  
  -- get the max
  pq4_max as (select Zi1, Zi, (Zi1 - Zi) * EXP(-1*ABS(i-0.9*9)) as Yi, i from pq_common),
  pq4sum_max as (select sum(Yi) as sumYi from pq4_max),
  pq5_max as (select *, Yi/sumYi as probYi, random() as rand from pq4_max cross join pq4sum_max),
  pq6_max as (select Zi1, Zi, i, rand < probYi as picked from pq5_max),
  pq6zero_max as (select min(Zi) as Zi1, 0 as Zi, 1 as i, true as picked from pq6_max),
  pq6with1_max as (select * from pq6_max union select * from pq6zero_max order by i asc),
  pq7_max as (select random()*(Zi1-Zi)+Zi as priv_max from pq6with1_max where picked is true order by i desc limit 1),
  
  -- get upper and lower clamping values
  crudes as (select (priv_max + priv_min)/2 as u_crude, ABS(priv_max - priv_min) as iqr_crude, POW((@* $n$ *@), 0.433) as rad from pq7_min cross join pq7_max),
  clamping_values as (select u_crude + 4 * rad * iqr_crude as upper, u_crude - 4 * rad * iqr_crude as lower from crudes)
SELECT upper as _<N>_upper, lower as _<N>_lower from clamping_values
\end{lstlisting}
\caption{Differentially Private Winsorized Mean in SQL}
\label{fig:winmean}
\end{figure*}
